# Supplementary material for: Attentional Prototype Inference for Few-Shot Segmentation
Source: arXiv:2105.06668 source file (2023-05-30)
Supplement: Supplementary file 1 [file 6-appendix.tex]

\appendix
\textbf{Derivations of the ELBO in (\ref{equa:1})}. For a single episode, we begin with maximizing log-likelihood conditional distribution $\log p(\mathbf{y}_q|\mathbf{x}_q,S)$ to derive the ELBO of API. By leveraging Jensen's inequality, we have the following steps as
\begin{align}
&\log p(\mathbf{y}_q|\mathbf{x}_q,S)   \nonumber\\%%%%%%1
&\; = \log \int \!\!\!\! \int p(\mathbf{y}_q|\mathbf{z},\mathbf{m}_q,\mathbf{x}_q)p(\mathbf{m}_q|\mathbf{x}_q)p(\mathbf{z}|\mathcal{S}) \;  d\mathbf{z}d\mathbf{m}_q   \label{eq_app:2}\\%%%%%%2 
&\; \geq \int  \log \Big [\int
 p(\mathbf{y}_q|\mathbf{z},\mathbf{m}_q,\mathbf{x}_q) p(\mathbf{z}|\mathcal{S})  \Big]\;  p(\mathbf{m}_q|\mathbf{x}_q)  \;      d\mathbf{z} d\mathbf{m}_q \label{eq_app:3}\\%%%%%%3
&\; \geq \int \!\!\!\! \int
\log \Big [ p(\mathbf{y}_q|\mathbf{z},\mathbf{m}_q,\mathbf{x}_q)\Big] p(\mathbf{z}|\mathcal{S})    p(\mathbf{m}_q|\mathbf{x}_q) \;      d\mathbf{z}  d\mathbf{m}_q  \label{eq_app:4} \\%%%%%%4
&\; = \int q_{\phi_2}(\mathbf{m}_q|\mathbf{x}_q,\mathbf{y}_q)   \int
 q_{\phi_1}(\mathbf{z}|\mathbf{x}_q,\mathbf{y}_q, \mathcal{S}) \nonumber \\ 
&\;\quad\quad\quad   \frac{\log \big[p(\mathbf{y}_q|\mathbf{z},\mathbf{m}_q,\mathbf{x}_q)\big] p(\mathbf{z}|\mathcal{S}) p(\mathbf{m}_q|\mathbf{x}_q)}{q_{\phi_1}(\mathbf{z}|\mathbf{x}_q,\mathbf{y}_q, \mathcal{S})
q_{\phi_2}(\mathbf{m}_q|\mathbf{x}_q,\mathbf{y}_q)}    \;      d\mathbf{z}d\mathbf{m}_q \label{eq_app:5}\\%%%%%%5
&\; = \int  \frac{q_{\phi_2}(\mathbf{m}_q|\mathbf{x}_q,\mathbf{y}_q) p(\mathbf{m}_q|\mathbf{x}_q)}{
q_{\phi_2}(\mathbf{m}_q|\mathbf{x}_q,\mathbf{y}_q)}  \nonumber\\
&\;\quad\quad\quad  E_{q_{\phi_1}(\mathbf{z}|\mathbf{x}_q,\mathbf{y}_q, \mathcal{S})} \log \big[p(\mathbf{y}_q|\mathbf{z},\mathbf{m}_q,\mathbf{x}_q)\big]\; d\mathbf{m}_q \nonumber\\ 
&\;\quad\quad\quad -D_{\mathrm{KL}}[q_{\phi_1}(\mathbf{z}|\mathbf{x}_q,\mathbf{y}_q, \mathcal{S})||p(\mathbf{z}|\mathcal{S})]  \label{eq_app:6}  \\%%%%%%6
& \quad = E_{q_{\phi_1}(\mathbf{z}|\mathbf{x}_q,\mathbf{y}_q, \mathcal{S}),q_{\phi_2}(\mathbf{m}_q|\mathbf{x}_q,\mathbf{y}_q)}\big[\log p(\mathbf{y}_q|\mathbf{z},\mathbf{m}_q,\mathbf{x}_q)\big] \nonumber\\
&\;\quad\quad\quad -D_{\mathrm{KL}}[q_{\phi_1}(\mathbf{z}|\mathbf{x}_q,\mathbf{y}_q, \mathcal{S})||p(\mathbf{z}|\mathcal{S})] \nonumber\\ &\;\quad\quad\quad-D_{\mathrm{KL}}[q_{\phi_2}(\mathbf{m}_q|\mathbf{x}_q,\mathbf{y}_q)||p(\mathbf{m}_q|\mathbf{x}_q)]. \label{eq_app:7}
\end{align}
We apply Jensen's inequality two times to obtain the two steps of (\ref{eq_app:3}) and (\ref{eq_app:4}). By introducing the two variational distributions of $q_{\phi_1}(\mathbf{z}|\mathbf{x}_q,\mathbf{y}_q, \mathcal{S})$ and $
q_{\phi_2}(\mathbf{m}_q|\mathbf{x}_q,\mathbf{y}_q)$, we can achieve the step (\ref{eq_app:5}). Since we assume $\mathbf{z}$ and $\mathbf{m}_q$ are independent, we have the ELBO \textit{w.r.t.} the variable $\mathbf{z}$ in (\ref{eq_app:6}). Finally, the ELBO in (\ref{equa:1}) is obtained.
